# Supplementary material for: Solvable model of driven matter with pinning
Source: arXiv:2306.09589 source file (2023-06-16)
Supplement: Supplementary file 1 [file supplemental-materials.pdf]

# Supplementary materials
# Solvable model of driven matter with pinning

Gourab Kumar Sar,[1] Dibakar Ghosh,[1] and Kevin O'Keeffe[2]

[1]*Physics and Applied Mathematics Unit, Indian Statistical Institute, 203 B. T. Road, Kolkata 700108, India*
[2]*Senseable City Lab, Massachusetts Institute of Technology, Cambridge, MA, USA, 02139*

## I. ANALYSIS FOR $N = 2$ PARTICLES

### A. $J = -K$ coupling

Our model is

$$\dot{x_1} = E - b\sin(x_1 - \alpha_1) + \frac{J}{2}\sin(x_2 - x_1)\cos(\theta_2 - \theta_1), \tag{S1}$$

$$\dot{x_2} = E - b\sin(x_2 - \alpha_2) - \frac{J}{2}\sin(x_2 - x_1)\cos(\theta_2 - \theta_1), \tag{S2}$$

$$\dot{\theta_1} = E - b\sin(\theta_1 - \beta_1) + \frac{K}{2}\sin(\theta_2 - \theta_1)\cos(x_2 - x_1), \tag{S3}$$

$$\dot{\theta_2} = E - b\sin(\theta_2 - \beta_2) - \frac{K}{2}\sin(\theta_2 - \theta_1)\cos(x_2 - x_1). \tag{S4}$$

Defining the difference and sum coordinates

$$x_\pm = \frac{x_1 \pm x_2}{2}, \tag{S5}$$

$$\theta_\pm = \frac{\theta_1 \pm \theta_2}{2}, \tag{S6}$$

and setting $(\alpha_1, \alpha_2) = (\beta_1, \beta_2) = (0, \pi)$, $b = 1$, and $J = -K$, we get

$$\dot{x}_+ = E - \cos x_+ \sin x_-, \tag{S7}$$

$$\dot{x}_- = -\sin x_+ \cos x_- + \frac{K}{2}\sin 2x_- \cos 2\theta_-, \tag{S8}$$

$$\dot{\theta}_+ = E - \cos\theta_+ \sin\theta_-, \tag{S9}$$

$$\dot{\theta}_- = -\sin\theta_+ \cos x_- - \frac{K}{2}\sin 2\theta_- \cos 2x_-, \tag{S10}$$

presented in the main text. To solve for the fixed points, we first eliminate $(x_-, \theta_-)$ using Eqs. (S7), (S9)

$$\sin x_- = E\sec x_+, \tag{S11}$$

$$\sin\theta_- = E\sec\theta_+. \tag{S12}$$

Subbing these into Eqs. (S8), (S10), we get

$$\sqrt{1 - E^2\sec^2 x_+}\Big(EK\sec x_+\left(2E^2\sec^2\theta_+ - 1\right) - \sin x_+\Big) = 0, \tag{S13}$$

$$\sqrt{1 - E^2\sec^2\theta_+}\Big(EK\sec\theta_+\left(2E^2\sec^2 x_+ - 1\right) - \sin\theta_+\Big) = 0. \tag{S14}$$

These have form $AB = CD = 0$ which imply four different fixed point defined by $(A, C), (A, D), (B, C), (B, D)$ being $(0, 0)$ individually.

**Pinned state**. The first correspond to the 'pinned' state defined by

$$\sqrt{1 - E^2\sec^2 x_+} = 0, \tag{S15}$$

$$\sqrt{1 - E^2\sec^2\theta_+} = 0. \tag{S16}$$

Which have solution

$$x_+ = \pm\cos^{-1} \pm E, \tag{S17}$$

$$x_- = \pm\frac{\pi}{2}, \tag{S18}$$

$$\theta_+ = \pm\cos^{-1} \pm E, \tag{S19}$$

$$\theta_- = \pm\frac{\pi}{2}. \tag{S20}$$

There are 16 total solutions, corresponding to the permutation induced by the various $\pm's$. Notice these only exist for $E \leq 1$. Only four are stable:

$$(x_+, x_-, \theta_+, \theta_-) = \Big(\cos^{-1}(-E), -\pi/2, \cos^{-1}(-E), -\pi/2\Big) \tag{S21}$$

$$= \Big(\cos^{-1}(-E), -\pi/2, -\cos^{-1}(E), \pi/2\Big) \tag{S22}$$

$$= \Big(-\cos^{-1}(E), \pi/2, \cos^{-1}(-E), -\pi/2\Big) \tag{S23}$$

$$= \Big(-\cos^{-1}(E), \pi/2, -\cos^{-1}(E), -\pi/2\Big) \tag{S24}$$

The eigenvalues are simply found using Mathematica:

$$\lambda = -\sqrt{1-E^2}, -\sqrt{1-E^2}, \sqrt{1-E^2} - K, \sqrt{1-E^2} - K. \tag{S25}$$

Recall the fixed points exist only when $E \leq 1$, which means the first two $\lambda$ are always negative. The second two become unstable via a zero eigenvalue bifurcation at

$$E_{c1} = \sqrt{1-K^2} \tag{S26}$$

as stated in the main text.

**Half-pinned state**. This state is defined by a symmetric pair of fixed points: when $x_i$ stay pinned and $\theta_i$ sync, or the reverse. In the above notation, these correspond to $(A, D) = (0, 0)$ and $(B, D) = (0, 0)$. We study the $(A, D) = (0, 0)$ without loss of generality, given by,

$$\sqrt{1 - E^2 \sec^2 x_+} = 0, \tag{S27}$$

$$\sqrt{1 - E^2 \sec^2 \theta_+}\Big(EK \sec\theta_+ \left(2E^2 \sec^2 x_+ - 1\right) - \sin\theta_+\Big) = 0. \tag{S28}$$

Mathematica finds 32 solutions to these, of which 4 are stable. These 4 fixed points have the form

$$x_+ = -\cos^{-1}(-E), \tag{S29}$$

$$x_- = -\frac{\pi}{2}, \tag{S30}$$

$$\theta_+ = \cos^{-1}\left(-\frac{\sqrt{1-\sqrt{1-4E^2K^2}}}{\sqrt{2}}\right), \tag{S31}$$

$$\theta_- = -\sin^{-1}\Big(\frac{\sqrt{2}E}{\sqrt{1-\sqrt{1-4E^2K^2}}}\Big). \tag{S32}$$

Finding the stability of these is harder. The Jacobian matrix yields eigenvalues

$$\lambda_1 = -\sqrt{1-E^2}, \tag{S33}$$

$$\lambda_2 = \frac{\sqrt{1-4E^2K^2} - K\left(\sqrt{1-E^2}+K\right)+1}{K}, \tag{S34}$$

$$\lambda_3 = \frac{1}{2}\left(-\frac{2E\sqrt{\sqrt{1-4E^2K^2}+1}}{\sqrt{1-\sqrt{1-4E^2K^2}}} - \frac{\sqrt{1-4E^2K^2}+\frac{\sqrt{K^2\left(8E^2\sqrt{1-4E^2K^2}-K^2\left(\sqrt{1-4E^2K^2}+16E^2-1\right)-4\sqrt{1-4E^2K^2}+4\right)}}{\sqrt{1-\sqrt{1-4E^2K^2}}}+1}{K}+K\right), \tag{S35}$$

$$\lambda_4 = \frac{1}{2}\left(-\frac{2E\sqrt{\sqrt{1-4E^2K^2}+1}}{\sqrt{1-\sqrt{1-4E^2K^2}}} - \frac{\sqrt{1-4E^2K^2}-\frac{\sqrt{K^2\left(8E^2\sqrt{1-4E^2K^2}-K^2\left(\sqrt{1-4E^2K^2}+16E^2-1\right)-4\sqrt{1-4E^2K^2}+4\right)}}{\sqrt{1-\sqrt{1-4E^2K^2}}}+1}{K}+K\right). \tag{S36}$$

Solving $\lambda_3 = 0$ and removing the square roots by successive squaring leads to

$$4E^4(2EK-1)(2EK+1)\left(E^2+K^2-1\right)\left(\left(2E^2K+K\right)^2+3\left(E^2-1\right)\right)=0. \tag{S37}$$

The relevant branch is

$$E_{c2} = -\frac{1}{2K}. \tag{S38}$$

Solving $\lambda_2 = 0$ gives us the other part of the boundary

$$E_{c3} = \frac{\sqrt{-K^4+5K^2-4}}{3K}. \tag{S39}$$

We again observe zero eigenvalue bifurcation on the boundary.

**Sync state**. The final fixed point $(B,D)=(0,0)$,

$$EK\sec x_+\left(2E^2\sec^2\theta_+-1\right)-\sin x_+=0, \tag{S40}$$

$$EK\sec\theta_+\left(2E^2\sec^2 x_+-1\right)-\sin\theta_+=0. \tag{S41}$$

Mathematica struggles solving these, so we have to do them by hand. First isolate $\sec\theta_+$ from the top equation

$$\sec\theta_+ = \frac{\sqrt{EK-\sin x_+\cos x_+}}{\sqrt{2}E^{3/2}\sqrt{K}}. \tag{S42}$$

Then sub this into the second equation after swapping $\sin\theta_+ = (1-1/\sec^2\theta_+)^{-1/2}$ to find

$$-\sqrt{K}\sqrt{2EK-\sin(2x_+)} - 2\sqrt{E}\sqrt{\frac{4E^3K}{\sin(2x_+)-2EK}+1} + 2E^2\sqrt{K}\sec^2(x_+)\sqrt{2EK-\sin(2x_+)} = 0. \tag{S43}$$

We remove the square roots by isolating each one on the LHS, squaring, then repeating the process. A gigantic equation in $\cos x_+, \sin x_+, \tan x_+$ results. Setting $c := \sqrt{\cos x_+}$ and simplifying however results in a product of a third and fourth order polynomials

$$P_3(c)P_4(c) = 0, \tag{S44}$$

where

$$P_3(c) = -c^3+c^4+c^2E^2K^2-4cE^4K^2+4E^6K^2, \tag{S45}$$

$$P_4(c) = c^4K^2+c^3\left(-8E^2K^2-K^2\right)+c^2\left(E^2K^4+16E^4K^2+4E^2K^2+4E^2\right)+c\left(-4E^4K^4-8E^4K^2\right)+4E^6K^4. \tag{S46}$$

Recalling $\cos x_+ = c^2$, we see $x_+$ will be a simple transformation of the roots of cubics and quartics – known, but ugly. These constitute a large family of fixed points. To find the relevant ones, we plotted them and found,

$$x_+ = \sec^{-1}\left(-\frac{2}{\sqrt{8E^2+\frac{S_2}{K}-S_1+1}}\right), \tag{S47}$$

$$x_- = -\sin^{-1}\left(\frac{2E}{\sqrt{8E^2+\frac{S_2}{K}-S_1+1}}\right), \tag{S48}$$

$$\theta_+ = -\cos^{-1}\left(\frac{2\sqrt{2}E^{3/2}\sqrt{K}}{\sqrt{\sqrt{-\frac{(8E^2K-KS_1+K+S_2)(S_2-K(-8E^2+S_1+3))}{K^2}}+4EK}}\right), \tag{S49}$$

$$\theta_- = \csc^{-1}\left(\frac{2\sqrt{2}\sqrt{E}\sqrt{K}}{\sqrt{\sqrt{-\frac{(8E^2K-KS_1+K+S_2)(S_2-K(-8E^2+S_1+3))}{K^2}}+4EK}}\right), \tag{S50}$$

where

$$S_1 = \sqrt{64E^4 - \frac{8E^2\left(K\left(K^2-2\right)\left(\sqrt{K^2-16E^2}+K\right)+2\right)}{K^2} + \frac{2\sqrt{K^2-16E^2}}{K}+2}, \tag{S51}$$

$$S_2 = \sqrt{K^2-16E^2}. \tag{S52}$$

Calculating the stability of these was another monster. We derived the characteristic equation which has form

$$a_4 + a_3\lambda + a_2\lambda^2 + a_1\lambda^3 + a_0\lambda^4 = 0, \tag{S53}$$

where $a_i = f_i(E, K)$ where $f$ were complicated functions.

$$a_0 = 1, \tag{S54}$$

$$a_1 = \frac{2\sqrt{1-E^2S_4^2}}{S_4} + 2E\sqrt{1-\frac{1}{S_3^2}}S_3, \tag{S55}$$

$$a_2 = \frac{K^2\left(S_4^4\left(-\left(1-2E^2S_3^2\right)^2\right)+4S_4^2-4\right)}{S_4^4} + \frac{K\left(S_4^2-2\right)\left(2E^2S_3^2-1\right)\left(\sqrt{1-E^2S_4^2}-E\sqrt{1-\frac{1}{S_3^2}}S_3S_4\right)}{S_4^3} + \frac{4E\sqrt{1-\frac{1}{S_3^2}}S_3\sqrt{1-E^2S_4^2}}{S_4} + E^2S_3^2 - E^2S_4^2 - \frac{1}{S_3^2} + \frac{1}{S_4^2}, \tag{S56}$$

$$a_3 = -\Bigg[K^2S_3^2\left(S_4^4\left(1-2E^2S_3^2\right)^2-4S_4^2+4\right)\left(\sqrt{1-E^2S_4^2}+E\sqrt{1-\frac{1}{S_3^2}}S_3S_4\right) + K\left(S_4^2-2\right)S_4\left(2E^2S_3^2-1\right)\left(S_3^2+S_4^2\right)\left(E^2S_3^2S_4^2-1\right) + 2S_4^3\left(E^3\sqrt{1-\frac{1}{S_3^2}}S_3^3S_4^4 - E^2S_3^4S_4\sqrt{1-E^2S_4^2} + S_4\sqrt{1-E^2S_4^2} - E\sqrt{1-\frac{1}{S_3^2}}S_3^3\right)\Bigg]\Bigg/ S_3^2S_4^5, \tag{S57}$$

$$
\begin{aligned}
a_4 = -\Bigg[ & - E^2 S_4^2 \left( S_3^4 \left( K S_4^2 \sqrt{1 - E^2 S_4^2} - 2K\sqrt{1 - E^2 S_4^2} + S_4 \right) + 2K S_3^2 \left( S_4^2 - 2 \right) \sqrt{1 - E^2 S_4^2} + S_4^5 \right) \\
& + EK\sqrt{1 - \frac{1}{S_3^2}} S_3^3 \left( S_4^2 - 2 \right) \left( K S_4^2 \sqrt{1 - E^2 S_4^2} - 2K\sqrt{1 - E^2 S_4^2} + S_4 \right) \\
& + S_4^2 \left( K S_4^2 \sqrt{1 - E^2 S_4^2} - 2K\sqrt{1 - E^2 S_4^2} + S_4 \right) + 2E^5 K\sqrt{1 - \frac{1}{S_3^2}} S_3^5 S_4^4 \left( 2K S_3^2 \sqrt{1 - E^2 S_4^2} + S_4^3 - 2S_4 \right) \\
& + E^4 S_3^4 S_4^2 \left( 2K S_3^2 S_4^2 \sqrt{1 - E^2 S_4^2} - 4K S_3^2 \sqrt{1 - E^2 S_4^2} + S_4^5 \right) - E^3 K\sqrt{1 - \frac{1}{S_3^2}} S_3^3 S_4 \Bigg( 2S_3^2 \left( 2K S_4^3 \sqrt{1 - E^2 S_4^2} + S_4^2 - 2 \right) \\
& + \left( S_4^2 - 2 \right) S_4^4 \Bigg) \Bigg] \Bigg/ S_3^2 S_4^5, \qquad \text{(S58)}
\end{aligned}
$$

where $S_3$ and $S_4$ are given by

$$
S_3 = \frac{2}{\sqrt{8E^2 + \frac{S_2}{K} - S_1 + 1}}, \qquad \text{(S59)}
$$

$$
S_4 = \frac{2\sqrt{2}\sqrt{E}\sqrt{K}}{\sqrt{\sqrt{-\frac{(8E^2K - KS_1 + K + S_2)(S_2 - K(-8E^2 + S_1 + 3))}{K^2}} + 4EK}}. \qquad \text{(S60)}
$$

The $\lambda$'s were findable in theory, but too complex to derive any meaningful stability information from. So instead checked the stability with the help of the Routh Hurwitz conditions:

$$
\begin{aligned}
a_0 &> 0, && \text{(S61)} \\
a_1 &> 0, && \text{(S62)} \\
a_1 a_2 - a_0 a_3 &> 0, && \text{(S63)} \\
(a_1 a_2 - a_0 a_3) a_3 - a_1^2 a_4 &> 0, && \text{(S64)} \\
a_4 &> 0. && \text{(S65)}
\end{aligned}
$$

We found that the sync state solutions Eqs. (S47)-(S50) are stable whenever they exist. They exist when the terms inside the square root in the expressions of $S_1$ and $S_2$ in Eqs. (S51) and (S52) are greater or equal to zero. This gives us the stability and existence boundaries of the sync state quoted in the main text

$$
E_{c4} = \frac{K}{4}, \qquad \text{(S66)}
$$

$$
E_{c5} = \frac{1}{2}\sqrt{\frac{K\left(\sqrt{K^2 - 4} + K\right) - 1}{K^2}}, \qquad \text{(S67)}
$$

### B. $J = +K$ coupling

The analysis here is the same dance as above, but surprisingly it gets easier. The governing equations read

$$
\begin{aligned}
\dot{x}_+ &= E - \cos x_+ \sin x_-, && \text{(S68)} \\
\dot{x}_- &= -\sin x_+ \cos x_- - \frac{K}{2} \sin 2x_- \cos 2\theta_-, && \text{(S69)} \\
\dot{\theta}_+ &= E - \cos\theta_+ \sin\theta_-, && \text{(S70)} \\
\dot{\theta}_- &= -\sin\theta_+ \cos x_- - \frac{K}{2} \sin 2\theta_- \cos 2x_-. && \text{(S71)}
\end{aligned}
$$

There are four fixed points like last time, but only the pinned and half-pinned are stable.

**Pinned**. The fixed points are

$$x_+ = \pm\cos^{-1}(\mp E), \tag{S72}$$
$$x_- = \pm\frac{\pi}{2}, \tag{S73}$$
$$\theta_+ = \pm\cos^{-1}(\mp E), \tag{S74}$$
$$\theta_- = \pm\frac{\pi}{2}. \tag{S75}$$

which has a saddle node at $E = \sqrt{1-K^2}$ ($K < 0$) and a sniper at $E = 1$ (Fig. S1). It is to be noted that, pinned state is the only stable steady solution for $K > 0$. The other steady state exists for $K < 0$ and we derive its stability next.

**Half pinned**. Here the fixed points are:

$$x_+ = \cos^{-1}(-E), \tag{S76}$$
$$x_- = -\frac{\pi}{2}, \tag{S77}$$
$$\theta_+ = \sec^{-1}\left(-\frac{\sqrt{2}}{\sqrt{1-\sqrt{1-4E^2K^2}}}\right), \tag{S78}$$
$$\theta_- = \sin^{-1}\left(\frac{\sqrt{2}E}{\sqrt{1-\sqrt{1-4E^2K^2}}}\right). \tag{S79}$$

We calculate the eigenvalues at this fixed point as

$$\lambda_1 = -\sqrt{1-E^2}, \tag{S80}$$
$$\lambda_2 = -\frac{K\left(\sqrt{1-E^2}-K\right)+S_3+1}{K}, \tag{S81}$$
$$\lambda_3 = \frac{1}{2}\left(-\frac{\frac{\sqrt{K^2(-K^2(16E^2+S_3-1)+8E^2S_3-4S_3+4)}}{\sqrt{1-S_3}}+S_3+1}{K}-\frac{2E\sqrt{S_3+1}}{\sqrt{1-S_3}}+K\right), \tag{S82}$$
$$\lambda_4 = \frac{1}{2}\left(-\frac{-\frac{\sqrt{K^2(-K^2(16E^2+S_3-1)+8E^2S_3-4S_3+4)}}{\sqrt{1-S_3}}+S_3+1}{K}-\frac{2E\sqrt{S_3+1}}{\sqrt{1-S_3}}+K\right). \tag{S83}$$

where

$$S_3 = \sqrt{1-4E^2K^2}, \tag{S84}$$
$$S_4 = \sqrt{K^2\left(8E^2\sqrt{1-4E^2K^2}-K^2\left(\sqrt{1-4E^2K^2}+16E^2-1\right)-4\sqrt{1-4E^2K^2}+4\right)}. \tag{S85}$$

Finally the stability boundary is found as

$$E_{c8} = -\frac{1}{2K}. \tag{S86}$$

At this boundary saddle node infinite period (SNIPER) bifurcation takes place which results into a periodic orbit. See Fig. S1. The black curves are the analytically calculated stability boundaries.

## II. CHAOS

We observe chaos in our model for both $J = -K$ and $J = K$.

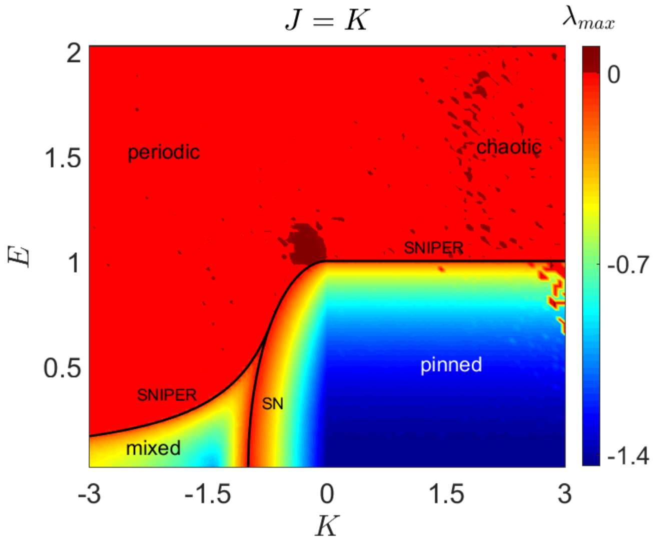


FIG. S1: Bifurcation diagrams in $(K, E)$ space with $J = K$ with largest Lyapunov exponent. Black curves denote analytically calculated stability boundaries. SN stands for saddle node bifurcation and SNIPER stands for saddle node infinite period bifurcation.

**Opposite sign coupling** $J = -K$. In Fig. S2, we analyze in detail the chaotic behavior by plotting the bifurcation diagram, power spectra, and time series for $J = -K$ with $N = 2$ swarmalators. Chaotic behavior emerges when the driving strength $E$ increases. The route is intermittent which can be seen from the power spectral density (PSD) plot. The chaotic attractor is demonstrated in Fig. S3 in the $\sin x_1$-$\sin x_2$ and $\sin\theta_1$-$\sin\theta_2$ planes.

**Same sign coupling** $J = K$**.** For $J = K$ and $N >> 1$ we observe show period doubling route to chaos. Here, the chaos is studied in terms of the order parameters $S_{\pm}$ defined by

$$W_{\pm} = S_{\pm} e^{\tilde{i}\Phi_{\pm}} = \frac{1}{N}\sum_j e^{\tilde{i}(x_j \pm \theta_j)} \quad (\tilde{i} = \sqrt{-1}). \tag{S87}$$

Figure S4 demonstrates the bifurcation diagram, largest Lyapunov exponents, and period doubling route to chaos.

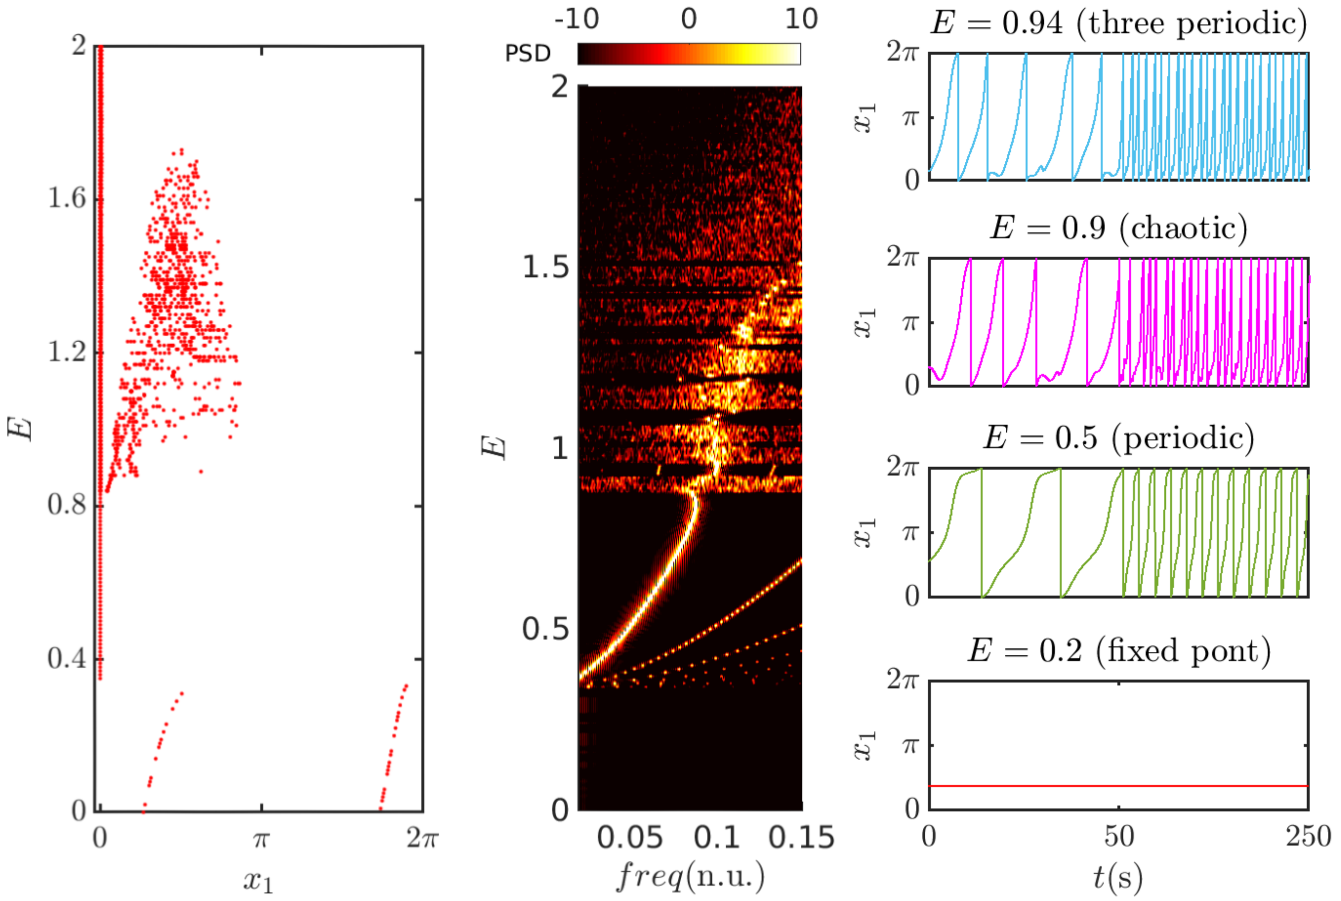


FIG. S2: Bifurcation diagram, power spectral density and time series. $K = -J = -1.5$. Simulation is performed with $N = 2$ swarmalators. For plotting the bifurcation diagram we have simulated our model for $T = 2000$ time units with step-size $dt = 0.01$ by RK4 method. Then last 5% data were considered and the local minimum are plotted. The same numerics were used for the PSD. The time series of $x_1$ are shown for four different values of $E$ over $T = 250$ time units starting from the initial time $t = 0$.

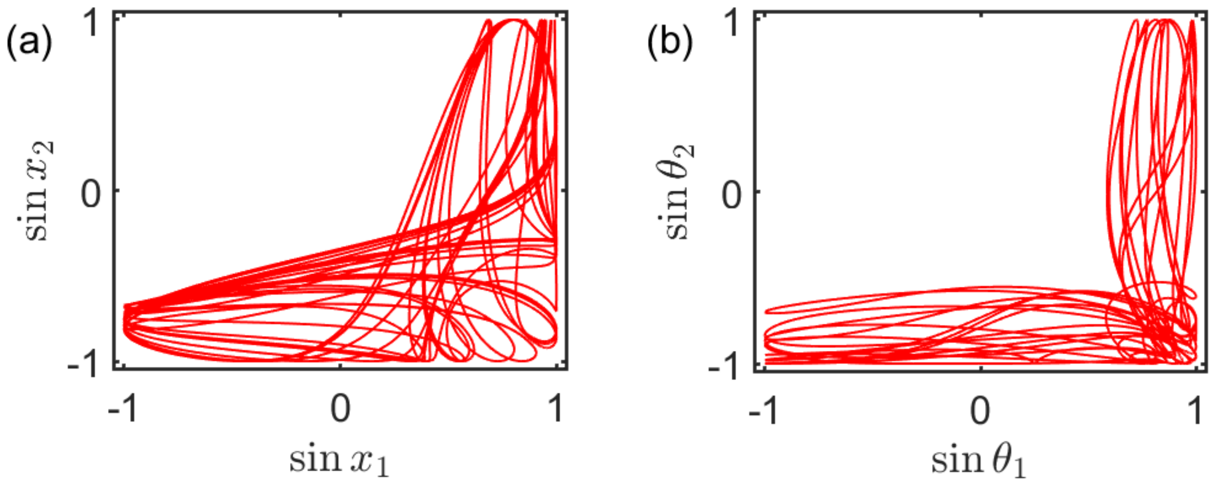


FIG. S3: Chaotic attractor at $K = -J = 1.5$, $E = 1.0$. The attractor is plotted with last 5% data after simulating the model for $T = 2000$ time units with step-size $dt = 0.01$ by RK4 method. (a) Projection on the $\sin x_1$-$\sin x_2$ plane. (b) Projection on the $\sin \theta_1$-$\sin \theta_2$ plane.

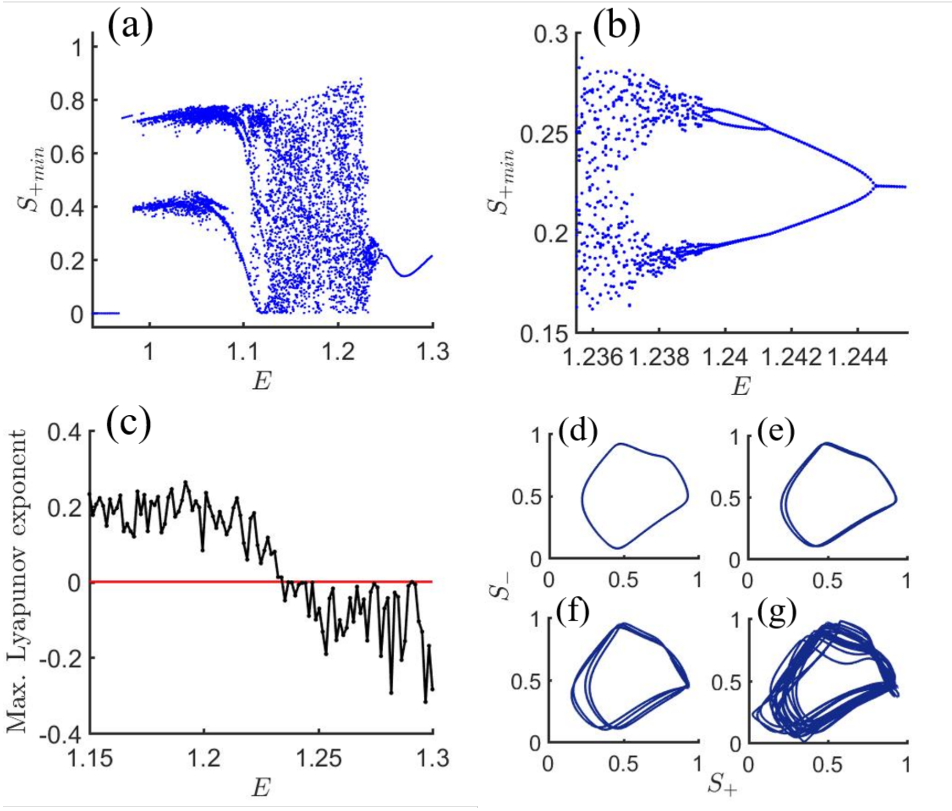


FIG. S4: Period doubling route to chaos for $J = K = 0.5$ and $N \gg 1$. (a) Bifurcations structure of $S_+(E)$. (b) Zoom in of inverse period doubling route to chaos. (c) Lyapunov exponents. (d)-(g) Period doubling illustrated in the $(S_+, S_-)$ plane. $E = 1.248, 1.243, 1.241, 1.23$ for the panels (d), (e), (f), and (g), respectively. In all panels, $K = 0.5$ and $(dt, T, N) = (0.01, 10000, 200)$. Last 20 % data were taken to calculate peaks of the time series of $S_+$.

## III. MODEL ROBUSTNESS

### A. When $J$ and $K$ have opposite signs but non-equal magnitude $J \neq -K$

We claimed in the main text that the line $J = -K$ captures the physics of the plane where $J$ and $K$ have opposite sign but different magnitude. Figure S5 illustrates this is the case. We study the model with $J = -\sqrt{3}K$ and $J = -K/\sqrt{3}$ which essentially show the same behavior as $J = -K$.

### B. Random / asymmetric pinning locations

In the main text, we chose symmetric $(\alpha_1, \alpha_2) = (0, \pi)$ for ease. Figure S6 shows that choosing $(\alpha_1, \alpha_2)$ randomly on $(0, \pi)$ does not change the overall physics. Without loss of generality, we make $\alpha_1 = 0$, take $\alpha_2 = a\pi$ and vary $a$ between 0 to 1. We find the existence of all the states for all values of $a$. Moreover, it also reveals that the half-pinned (blue region) and sync (green region) states are reentrant. In Fig. S7, we show that the largest Lyapunov exponent remains invariant when we change $a$. (Note this is all for the opposite sign case study $J = -K$).

## IV. REALISTIC VELOCITY-FORCE CURVES

The force velocity curve $\bar{v}(E)$ is a standard way to catalog the behavior of a pinned-driven systems. There are many types of $\bar{v}$ observed in nature; we recommend reading [S1] for a review. Figure S9 shows our model can imitate one of the more exotic $\bar{v}(E)$ curves, that observed for pinned superconductor vortices.

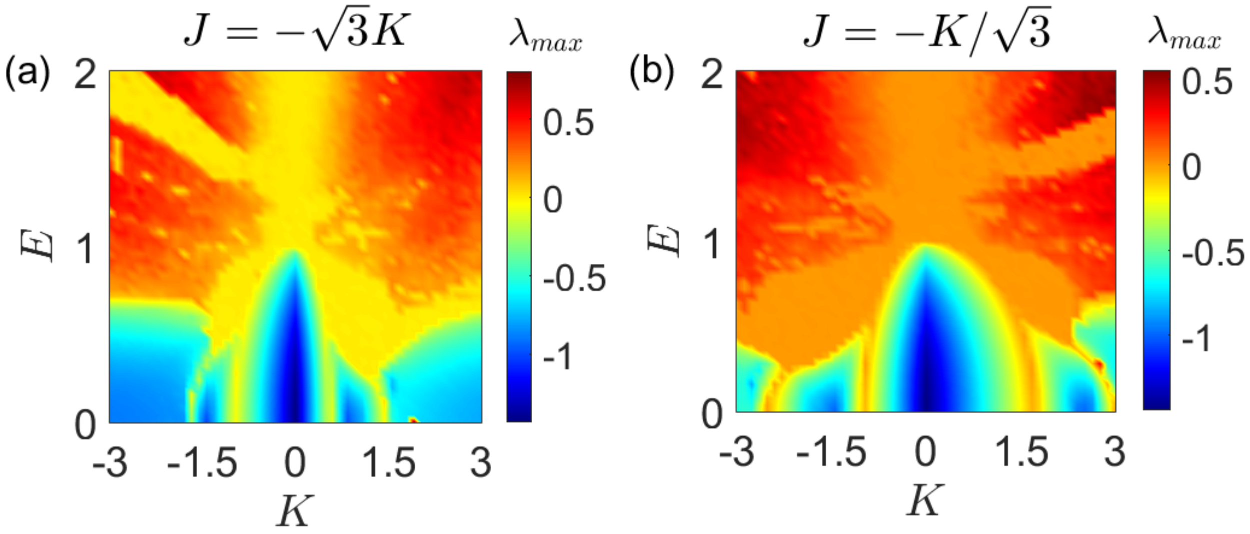


FIG. S5: Bifurcation diagrams in $(K, E)$ space with (a) $J = -\sqrt{3}K$ and (b) $J = -K/\sqrt{3}$.

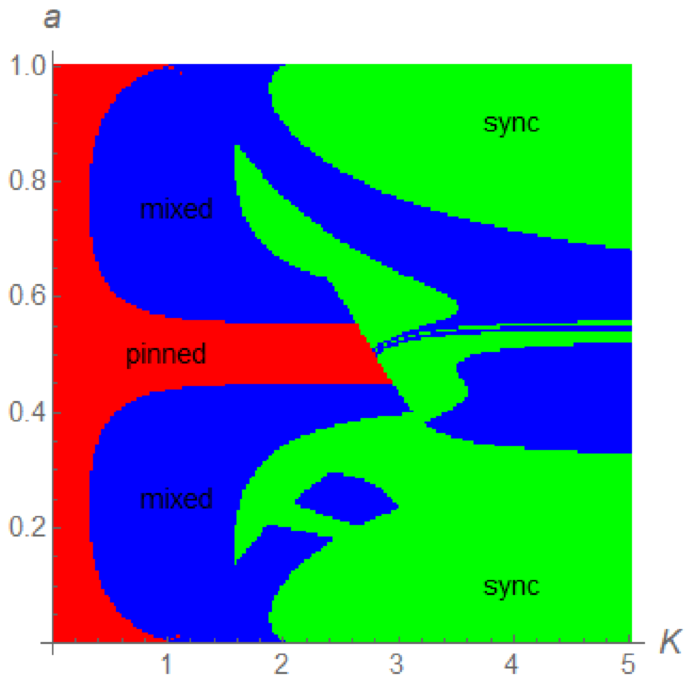


FIG. S6: Pinning locations $(\alpha_1, \alpha_2) = (\beta_1, \beta_2) = (0, a\pi)$ where $a$ varies between $[0, 1]$. $J = -K$. $E = 0.1$.


[S1] C. Reichhardt and C. O. Reichhardt, Reports on Progress in Physics **80**, 026501 (2016).

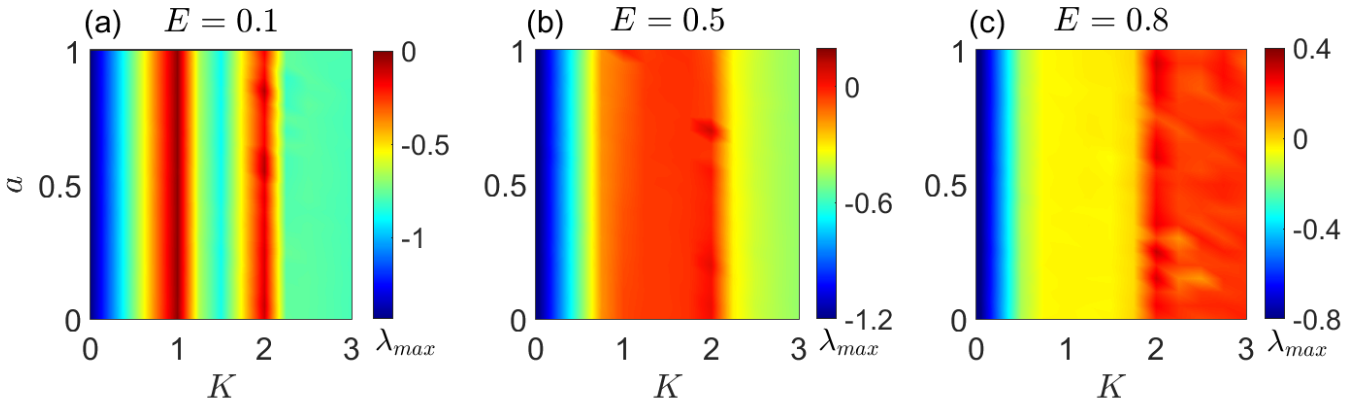


FIG. S7: Largest Lyapunov exponent. Pinning locations $(\alpha_1, \alpha_2) = (\beta_1, \beta_2) = (0, a\pi)$ where $a$ varies between $[0, 1]$. $J = -K$. (a) $E = 0.1$, (b) $E = 0.5$, (c) $E = 0.8$.

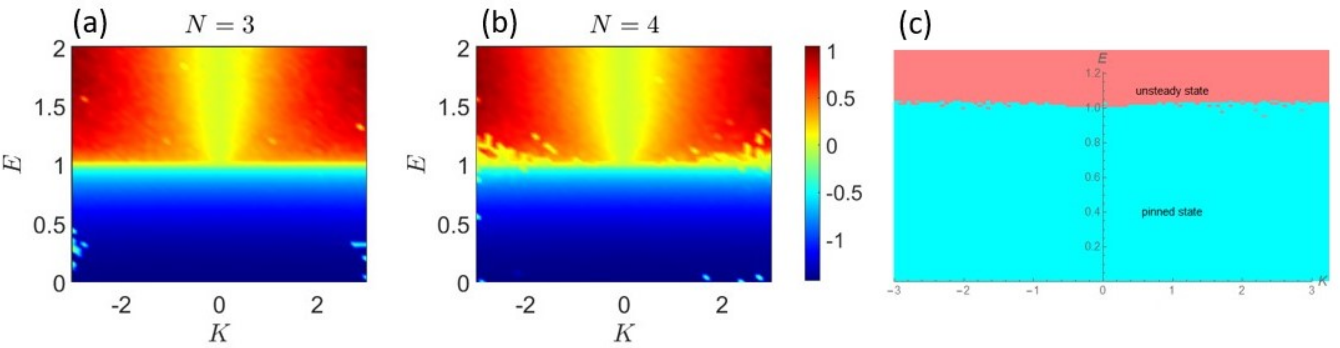


FIG. S8: $J = -K$. $K$-$E$ space for (a) $N = 3$, (b) $N = 4$, and (c) $N \gg 1$. Notice the $N = 3, 4$ plots are much different to the $N = 2$ plot shown in the main text. Instead, they resemble the $N \to \infty$ plot (c).

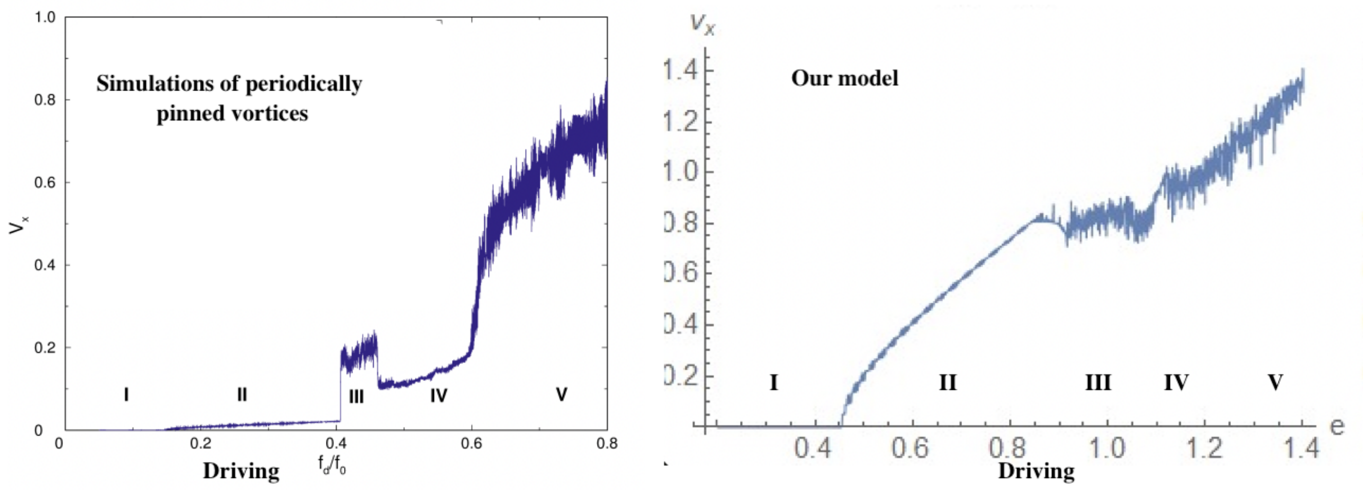


FIG. S9: Comparison of velocity-force curves $\bar{v}_x(E)$ from realistic simulations of superconducting vortices and our model. Left: adapted from [S1] (Figure 31); notice here the driving / force is denoted by $f_d/f_0$. Hysteresis is also observed but not plotted. Right: our model with $(dt, T, N) = (0.1, 200, 2)$ for $J = -K = -1.1$. The average velocity is over the $x-$velocity only (to facilitate a better comparison with simulations, which only plot $v_x$). Roman numerals mark regions of qualitatively different behavior, such as pinned, periodic, and chaotic states; see [S1] Section 6 titled "Depinning and Dynamic Phases on Periodic Pinning Arrays". Figure reproduced with permission from [S1].

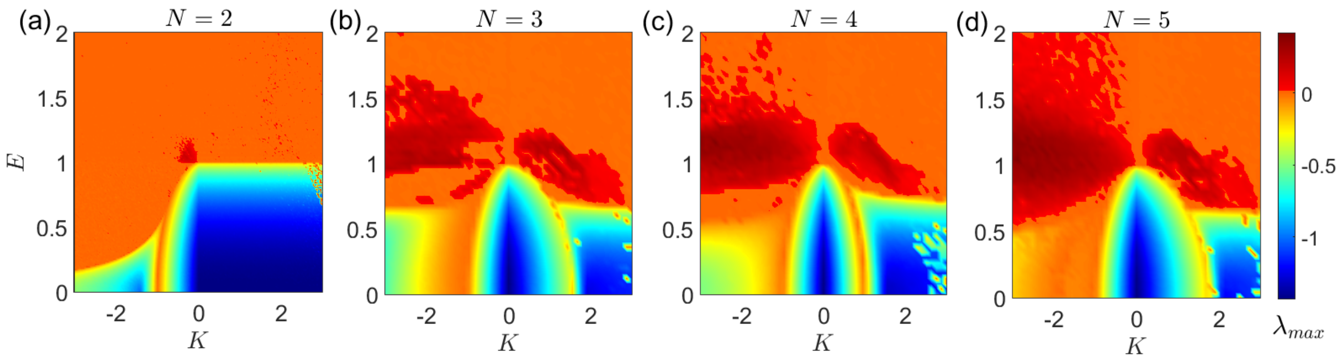


FIG. S10: Comparison of $N = 2, 3, 4, 5$ for $J = K$. As $N$ increases, the shape starts to change. At $N = 5$ the shape is almost identical to that of the $N = \infty$ results, plotted in Figure S11 below for convenience.

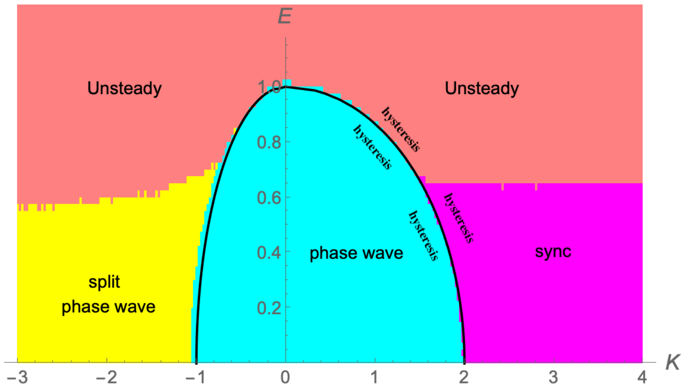


FIG. S11: Bifurcation diagram: $N \gg 1$ for $J = K$. We take $N = 100$ here.
